# Supplementary material for: Elastic alpha scattering experiments and the alpha-nucleus optical potential at low energies
Source: arXiv:1212.2891 source file (2012-12-12)
Supplement: Supplementary file 1 [file sm144a_exp.tex]

15.023 & 9.9443e-01 & 1.1358e-02    &   81.188 & 8.2501e-01 & 1.1285e-02  &  149.154 & 1.5125e-01 & 1.9187e-03 \\
  16.050 & 1.0003e+00 & 1.1369e-02    &   82.193 & 8.0272e-01 & 8.5563e-03  &  151.106 & 1.4843e-01 & 2.3744e-03 \\
  17.076 & 9.9475e-01 & 1.1447e-02    &   83.197 & 7.8205e-01 & 8.4548e-03  &  153.057 & 1.4558e-01 & 1.7674e-03 \\
  18.103 & 9.9632e-01 & 1.1476e-02    &   84.201 & 7.7795e-01 & 8.4650e-03  &  155.007 & 1.4175e-01 & 1.5249e-03 \\
  19.129 & 1.0040e+00 & 1.1373e-02    &   85.204 & 7.5133e-01 & 8.2115e-03  &  156.957 & 1.4222e-01 & 1.7300e-03 \\
  20.156 & 1.0128e+00 & 1.1000e-02    &   86.207 & 7.3524e-01 & 7.9127e-03  &  158.905 & 1.3723e-01 & 1.5221e-03 \\
  21.182 & 1.0036e+00 & 1.0368e-02    &   87.210 & 7.1104e-01 & 7.7805e-03  &  160.853 & 1.3005e-01 & 1.6623e-03 \\
  22.208 & 9.9883e-01 & 1.0315e-02    &   88.211 & 6.9320e-01 & 7.6758e-03  &  162.123 & 1.2510e-01 & 1.9469e-03 \\
  23.233 & 9.9291e-01 & 1.0266e-02    &   89.213 & 6.6963e-01 & 7.2226e-03  &  162.801 & 1.2879e-01 & 1.6782e-03 \\
  24.259 & 1.0037e+00 & 1.0246e-02    &   90.214 & 6.4842e-01 & 7.2072e-03  &  164.747 & 1.3078e-01 & 1.4544e-03 \\
  25.284 & 9.9131e-01 & 1.0209e-02    &   91.214 & 6.4119e-01 & 7.3793e-03  &  166.694 & 1.3469e-01 & 1.5707e-03 \\
  26.309 & 1.0053e+00 & 1.0339e-02    &   92.214 & 6.2289e-01 & 6.9926e-03  &  168.639 & 1.3041e-01 & 1.5328e-03 \\
  27.334 & 1.0085e+00 & 1.0550e-02    &   93.213 & 5.9840e-01 & 6.8849e-03  &  170.585 & 1.1894e-01 & 1.7970e-03 \\
  28.359 & 1.0027e+00 & 1.0288e-02    &   94.213 & 5.8820e-01 & 6.8378e-03  &  171.852 & 1.2050e-01 & 1.9303e-03 \\
  29.384 & 1.0066e+00 & 1.0497e-02    &   95.211 & 5.7078e-01 & 6.6741e-03  &  172.530 & 1.2304e-01 & 1.9399e-03 \\
  30.408 & 1.0198e+00 & 1.5073e-02    &   96.209 & 5.5617e-01 & 6.3424e-03 \\
  31.432 & 1.0206e+00 & 1.0765e-02    &   97.207 & 5.4371e-01 & 6.3622e-03 \\
  32.456 & 1.0133e+00 & 1.0700e-02    &   98.204 & 5.2301e-01 & 6.2452e-03 \\
  33.480 & 1.0101e+00 & 1.0703e-02    &   99.200 & 5.0597e-01 & 5.7763e-03 \\
  34.503 & 1.0028e+00 & 1.0409e-02    &  100.196 & 4.8451e-01 & 5.8156e-03 \\
  35.526 & 9.9627e-01 & 1.0516e-02    &  101.192 & 4.7642e-01 & 5.1353e-03 \\
  36.549 & 9.9647e-01 & 1.0504e-02    &  102.187 & 4.5164e-01 & 5.0754e-03 \\
  37.571 & 9.8968e-01 & 1.0777e-02    &  103.181 & 4.3703e-01 & 4.8139e-03 \\
  38.593 & 9.7495e-01 & 1.0256e-02    &  104.176 & 4.2290e-01 & 4.7648e-03 \\
  39.615 & 9.6950e-01 & 1.0532e-02    &  105.169 & 4.1079e-01 & 4.6410e-03 \\
  40.637 & 9.6466e-01 & 9.7744e-03    &  106.162 & 3.9585e-01 & 4.4592e-03 \\
  41.658 & 9.7528e-01 & 9.8899e-03    &  107.155 & 3.8909e-01 & 4.3815e-03 \\
  42.679 & 9.7642e-01 & 9.8882e-03    &  108.147 & 3.7559e-01 & 4.2371e-03 \\
  43.700 & 9.8185e-01 & 9.8995e-03    &  109.139 & 3.7004e-01 & 4.1823e-03 \\
  44.720 & 9.9564e-01 & 1.0739e-02    &  110.131 & 3.5743e-01 & 4.0724e-03 \\
  45.740 & 9.9389e-01 & 1.0787e-02    &  111.122 & 3.5313e-01 & 4.4442e-03 \\
  46.760 & 1.0090e+00 & 1.0321e-02    &  112.112 & 3.4082e-01 & 4.1145e-03 \\
  47.779 & 1.0311e+00 & 1.0710e-02    &  113.102 & 3.2933e-01 & 3.8544e-03 \\
  48.798 & 1.0241e+00 & 1.0427e-02    &  114.091 & 3.2274e-01 & 3.8990e-03 \\
  49.816 & 1.0356e+00 & 1.0619e-02    &  115.081 & 3.1234e-01 & 3.7879e-03 \\
  50.834 & 1.0309e+00 & 1.4915e-02    &  116.069 & 3.0205e-01 & 3.6464e-03 \\
  51.852 & 1.0264e+00 & 1.0540e-02    &  117.057 & 2.9361e-01 & 3.5441e-03 \\
  52.870 & 1.0372e+00 & 1.0619e-02    &  118.045 & 2.8855e-01 & 3.4788e-03 \\
  53.887 & 1.0473e+00 & 1.0634e-02    &  119.032 & 2.8037e-01 & 3.4015e-03 \\
  54.904 & 1.0615e+00 & 1.2113e-02    &  120.019 & 2.7391e-01 & 3.3467e-03 \\
  55.920 & 1.0585e+00 & 1.2193e-02    &  121.006 & 2.6823e-01 & 3.0816e-03 \\
  56.936 & 1.0729e+00 & 1.1172e-02    &  121.992 & 2.6231e-01 & 3.3439e-03 \\
  57.951 & 1.0859e+00 & 1.1612e-02    &  122.977 & 2.5435e-01 & 3.2114e-03 \\
  58.966 & 1.0707e+00 & 1.1058e-02    &  123.963 & 2.4514e-01 & 3.1427e-03 \\
  59.981 & 1.0765e+00 & 1.1256e-02    &  124.947 & 2.4257e-01 & 3.0962e-03 \\
  60.995 & 1.0784e+00 & 1.2439e-02    &  125.932 & 2.3291e-01 & 2.9983e-03 \\
  62.009 & 1.0856e+00 & 1.1070e-02    &  126.916 & 2.2770e-01 & 2.9369e-03 \\
  63.023 & 1.0811e+00 & 1.1102e-02    &  127.899 & 2.2438e-01 & 2.8588e-03 \\
  64.036 & 1.0562e+00 & 1.0887e-02    &  128.883 & 2.1325e-01 & 2.7834e-03 \\
  65.048 & 1.0508e+00 & 1.0674e-02    &  129.865 & 2.0998e-01 & 2.7413e-03 \\
  66.060 & 1.0530e+00 & 1.0896e-02    &  130.848 & 2.0899e-01 & 2.4601e-03 \\
  67.072 & 1.0813e+00 & 1.1394e-02    &  131.830 & 2.0525e-01 & 2.8782e-03 \\
  68.083 & 1.0539e+00 & 1.1141e-02    &  132.812 & 1.9583e-01 & 2.7198e-03 \\
  69.094 & 1.0510e+00 & 1.1155e-02    &  133.793 & 1.9263e-01 & 2.7122e-03 \\
  70.105 & 1.0272e+00 & 1.0848e-02    &  134.774 & 1.8840e-01 & 2.6513e-03 \\
  71.114 & 9.9017e-01 & 1.9709e-02    &  135.755 & 1.8559e-01 & 2.6127e-03 \\
  72.124 & 9.5337e-01 & 9.8877e-03    &  136.735 & 1.8482e-01 & 2.6003e-03 \\
  73.133 & 9.7721e-01 & 1.0268e-02    &  137.715 & 1.7488e-01 & 2.3660e-03 \\
  74.141 & 9.3970e-01 & 9.9395e-03    &  138.695 & 1.7477e-01 & 2.4885e-03 \\
  75.150 & 9.0827e-01 & 9.3548e-03    &  139.674 & 1.7163e-01 & 2.4374e-03 \\
  76.157 & 9.0651e-01 & 9.6564e-03    &  140.653 & 1.7070e-01 & 2.4102e-03 \\
  77.164 & 9.4688e-01 & 1.0412e-02    &  141.334 & 1.7327e-01 & 2.5866e-03 \\
  78.171 & 9.0078e-01 & 9.9673e-03    &  143.291 & 1.6624e-01 & 2.6274e-03 \\
  79.177 & 8.8001e-01 & 9.8128e-03    &  145.246 & 1.6039e-01 & 2.0330e-03 \\
  80.183 & 8.7745e-01 & 9.6887e-03    &  147.201 & 1.5589e-01 & 1.9312e-03 \\
